# Supplementary material for: AdaIR: Exploiting Underlying Similarities of Image Restoration Tasks with Adapters
Source: arXiv:2404.11475 source file (2024-04-17)
Supplement: Supplementary file 1 [file appendix.tex]

\newpage
\appendix

\setcounter{section}{0}
\setcounter{equation}{0}
\setcounter{figure}{0}
\setcounter{table}{0}

%%%%%%%%% SUPPLEMENTARY MATERIALS
\section{Supplementary Material}
\label{sec::supp_material}
This supplementary material is organized as follows.
Section~\ref{sec::supp_unet} demonstrates the flexibility of the foundation model in our \modelname~framework.
Section~\ref{sec::supp_real} presents additional results on real datasets. Section~\ref{sec::supp_exp} provides further experimental results of \modelname~. Finally, the limitations of our proposed \modelname~are summarized in Section~\ref{sec::supp_limitations}.    

%%%%%%%%% LIST of NOTATIONS
\subsection{List of Notations}
\label{sec::supp_notations}
In this section, the list of notations used throughout the main manuscript and supplementary materials are provided. The symbols and their corresponding definitions are summarized in Table~\ref{table::notations}.
\begin{table}[ht]
\centering
\footnotesize
\resizebox{\linewidth}{!}{
\begin{tabular}{l|l} 
\specialrule{0.8pt}{0.0ex}{0.0ex}
\textbf{Symbol}     & \textbf{Description} \\ 
\specialrule{0.8pt}{0.0ex}{0.0ex}
$r$                 & The index of the restoration tasks \\
$b$                 & The index of adapter blocks \\
$l$                 & The index of adapter layers \\ 
\specialrule{0.8pt}{0.0ex}{0.0ex}
$E$                 & Easy subsets \\
$H$                 & Hard subsets \\ 
\specialrule{0.8pt}{0.0ex}{0.0ex}
Unet$_E$            & Unet trained with easy subsets of multiple restoration tasks \\
Unet$_{E+H}$        & Unet trained with easy and hard subsets of multiple restoration tasks \\ 
Unet-S$_E$          & Unet trained with an easy subset of single restoration task \\
Unet-S$_{E+H}$      & Unet trained with easy and hard subsets of single restoration task \\ 
\specialrule{0.8pt}{0.0ex}{0.0ex}
Restormer$_E$       & Restormer trained with easy subsets of multiple restoration tasks \\
Restormer$_{E+H}$   & Restormer trained with easy and hard subsets of multiple restoration tasks \\
Restormer-S$_E$     & Restormer trained with an easy subset of single restoration task \\
Restormer-S$_{E+H}$ & Restormer trained with easy and hard subsets of single restoration task \\ 
\specialrule{0.8pt}{0.0ex}{0.0ex}
PromptIR$_E$        & PromptIR trained with easy subsets of multiple restoration tasks \\
PromptIR$_{E+H}$    & PromptIR trained with easy and hard subsets of multiple restoration tasks \\
PromptIR-S$_E$      & PromptIR trained with an easy subset of single restoration task \\
PromptIR-S$_{E+H}$  & PromptIR trained with easy and hard subsets of single restoration task \\ 
\specialrule{0.8pt}{0.0ex}{0.0ex}
\multirow{2}{*}{AdaIR} & AdaIR fine-tuned with hard subset of target restoration task \\
& with frozen foundation model trained by easy subsets of multiple restorations tasks \\
\specialrule{0.8pt}{0.0ex}{0.0ex}
\multirow{2}{*}{AdaIR-S} & AdaIR fine-tuned with hard subset of target restoration task \\
& with frozen foundation model trained by an easy subset of single restorations task \\
\specialrule{0.8pt}{0.0ex}{0.0ex}
\end{tabular}
}
\caption{The list of notations.}
\label{table::notations}
\vspace{-15pt}
\end{table}

%%%%%%%%% FOUNDATION MODEL
\subsection{Varient Architectures of Foundation Models}
\label{sec::supp_unet}
The objective of \modelname~is to integrate a lightweight adapter module into a foundation model, which enables rapid adaptation to downstream tasks previously unseen by the model. This strategy allows the foundation model to generalize across multiple specific restoration tasks without incurring the substantial memory consumption associated with maintaining separate foundation models for each task. In \modelname, the architecture of the foundation model remains flexible, as the adapter module is a plug-and-play component that can be easily incorporated into various deep models. This flexibility implies that we can interchange different types of deep models as our foundation model.

Most prior works focus on incorporating adapter modules within the Transformer block, both in high-level vision and NLP domains. In the main manuscript, we have chosen the architecture proposed in Restormer~\cite{restormer} as our foundation model, which is a classic Transformer-based deep model. Here, we replace the foundation model with Unet~\citesupp{unet}, renowned for its generality, flexibility, and scalability. Unlike Restormer~\cite{restormer}, the vintage Unet model does not involve Transformer blocks; instead, it comprises various convolutional layers within a multi-level hierarchical structure.

In recent years, the Unet architecture has been extensively developed for image segmentation, recognition, and other vision tasks. Additionally, the popular diffusion model DDPM~\citesupp{ddpm} also adopts Unet as its reconstruction model. Specifically, we utilize the Unet configuration employed by DDPM. Rather than merely processing the latent embeddings through convolutional layers, residual connections are introduced into the architecture. Consequently, our Unet foundation model consists of several residual blocks arranged in an encoder-decoder multi-level hierarchical structure. To integrate the adapter module into the Unet foundation model, we insert the adapter modules within the residual blocks, which is similar to their placement in Transformer blocks.

\begin{table}[t]
\centering
\footnotesize
\resizebox{\linewidth}{!}{
\begin{tabular}{l|P{10mm}P{12mm}|P{10mm}P{12mm}|P{10mm}P{10mm}|P{10mm}P{10mm}|P{10mm}P{10mm}|P{10mm}P{10mm}|P{20mm}}
\multirow{3}{*}{Method} & \multicolumn{4}{c|}{Gaussian Denoising}                      & \multicolumn{4}{c|}{Super-Resolution}                     & \multicolumn{4}{c|}{Gaussian Deblurring}                          & Deraining       \\ 
\cline{2-14}
                        & \multicolumn{2}{c|}{BSD68~\cite{bsd68}} & \multicolumn{2}{c|}{Urban100~\cite{urban100}} & \multicolumn{2}{c|}{B100~\cite{b100}} & \multicolumn{2}{c|}{Urban100~\cite{urban100}} & \multicolumn{2}{c|}{BSD68~\cite{bsd68}}     & \multicolumn{2}{c|}{Urban100~\cite{urban100}}  & Rain100H~\cite{rain100l} \\
                        & $\sigma=70$ & $\sigma=100$  & $\sigma=70$ & $\sigma=100$     & $\times 6$ & $\times 8$   & $\times 6$ & $\times 8$       & \textit{k19s4} & \textit{k21s5} & \textit{k19s4} & \textit{k21s5} & \textit{heavy}  \\ 
\specialrule{0.8pt}{0.0ex}{0.0ex}
Unet$_E$~\citesupp{unet}        & 21.38         & 15.93         & 21.64         & 16.00         & 23.54         & 23.66         & 21.00         & 20.56         & 23.45         & 22.42         & 20.37         & 19.35         & 16.34           \\
Unet$_{E+H}$~\citesupp{unet}    & \bu{26.78}    & \bu{25.33}    & \bu{26.98}    & \bu{25.30}    & \bu{25.76}    & \bu{24.72}    & \bu{23.48}    & \bu{21.30}    & \bu{26.77}    & \bu{25.46}    & \bu{24.39}    & \bu{22.76}    & \rb{29.87}           \\
AdaIR-Unet                      & \rb{26.81}    & \rb{25.36}    & \rb{27.07}    & \rb{25.34}    & \rb{25.76}    & \rb{24.73}    & \rb{23.50}    & \rb{22.04}    & \rb{26.99}    & \rb{25.60}    & \rb{24.75}    & \rb{22.95}    & \bu{29.19}          
\end{tabular}
}
\caption{The average PSNR (dB) over the hard subsets of the restoration tasks including Gaussian denoising, super-resolution, Gaussian deblurring, and deraining. The best and second-best performing results are highlighted by the \rb{red} and \bu{blue} colors, respectively.}
\vspace{-25pt}
\label{table::unet_results}
\end{table}

We conduct experiments on the four restoration tasks introduced in the main manuscript, maintaining the same training settings, except that the foundation model is switched from Restormer~\cite{restormer} to Unet~\citesupp{unet}. Table~\ref{table::unet_results} summarizes the quantitative results in terms of PSNR (dB) for Gaussian denoising, super-resolution, Gaussian deblurring, and deraining tasks. Specifically, the hard subsets of each task serve as the restoration target, with Unet$_E$ trained on the easy subsets, and Unet$_{E+H}$ trained on a mixed set of easy and hard subsets.

In Table~\ref{table::unet_results}, our proposed $\text{AdaIR-Unet}$ is fine-tuned from Unet$_E$. The evaluation results for Unet$_E$ indicate that the foundation model performs poorly on degradations not encountered during its training. However, with the injection of adapter modules and subsequent fine-tuning for downstream tasks, $\text{AdaIR-Unet}$ shows improvements in evaluation results compared to Unet$_E$. This improvement demonstrates that our proposed method can effectively adapt the foundation model to specific tasks. Furthermore, $\text{AdaIR-Unet}$ achieves comparable or even superior results against the Unet$_{E+H}$ setting. These findings validate the effectiveness of our method, which can be applied to foundation models beyond those based on the Transformer architecture. Moreover, compared to Unet$_{E+H}$, our approach requires training only a few parameters within the adapter modules, not the entire model. This efficiency enables the storage of a single foundation model with various adapter modules to handle multiple degradations, eliminating the need to duplicate the large foundation model multiple times.

%%%%%%%%% REAL ENVIRONMENTS
\subsection{Extension to Real Environments}
\label{sec::supp_real}

\begin{table}[t]
    \centering
    \footnotesize
    \begin{minipage}[ht]{0.49\linewidth}
        \centering
        \footnotesize
        \resizebox*{1\linewidth}{!}{
        \begin{tabular}{l|P{12mm}P{12mm}P{12mm}}
        \multirow{2}{*}{Method} & \multicolumn{3}{c}{SIDD~\citesupp{sidd}} \\
         & PSNR $\uparrow$ & SSIM $\uparrow$ & Time $\downarrow$ \\ 
        \specialrule{0.8pt}{0.0ex}{0.0ex}
        Input & 23.66 & 0.334 & - \\
        \specialrule{0.8pt}{0.0ex}{0.0ex}
        Restormer$_E$       & 23.92 & 0.341 & 43hr\\
        Restormer-S$_{E}$   & 26.25 & 0.464 & 15hr \\
        PromptIR$_E$        & 23.92 & 0.342 & 48hr\\
        PromptIR-$S_{E}$    & 26.15 & 0.460 & 27hr \\
        \specialrule{0.8pt}{0.0ex}{0.0ex}
        % Restormer$^\dag$ & 40.02 & 0.960 & - \\
        AdaIR$_E$           & \bu{38.84} & \bu{0.913} & 5hr \\
        AdaIR-$S_{E}$       & \rb{38.92} & \rb{0.914} & 5hr
        \end{tabular}
        }
        \caption{The average PSNR (dB) on SIDD dataset~\protect\citesupp{sidd}. The best and second-best performing results are highlighted by the \rb{red} and \bu{blue} colors, respectively.}
        \label{table::sidd_results}
        \vspace{-20pt}
    \end{minipage}
    \begin{minipage}[ht]{0.49\linewidth}
        \centering
        \footnotesize
        \resizebox*{1\linewidth}{!}{
        \begin{tabular}{l|P{12mm}P{12mm}P{12mm}}
        \multirow{2}{*}{Method} & \multicolumn{3}{c}{RealSR $\times 4$~\citesupp{realsr}} \\
         & PSNR $\uparrow$ & SSIM $\uparrow$ & Time \\ 
        \specialrule{0.8pt}{0.0ex}{0.0ex}
        Bicubic             & 27.99 & 0.806 & - \\
        \specialrule{0.8pt}{0.0ex}{0.0ex}
        Restormer$_E$       & 27.74 & 0.784 & 43hr \\
        Restormer-S$_{E}$   & 27.87 & 0.787 & 15hr \\
        PromptIR$_E$        & 27.69 & 0.782 & 48hr \\
        PromptIR-$S_{E}$    & 27.87 & 0.787 & 28hr \\
        \specialrule{0.8pt}{0.0ex}{0.0ex}
        % RealSR$^\dag$ & 28.92 & 0.834 & - \\
        AdaIR$_E$           & \rb{29.55} & \rb{0.835} & 2hr \\
        AdaIR-S$_E$         & \bu{29.48} & \bu{0.833} & 2hr \\
        \end{tabular}
        }
        \caption{The average PSNR (dB) on RealSR dataset~\protect\citesupp{realsr} with a scaling factor of 4. The best and second-best performing results are highlighted by the \rb{red} and \bu{blue} colors, respectively.}
        \label{table::realsr_results}
        \vspace{-20pt}
    \end{minipage}
\end{table}
In the main manuscript, all experiments are conducted within synthetic environments, which involve generating noisy, blurry, rainy, and LR images. While controllable configurations provide a stable platform for validating the efficacy of our proposed method, its capability to restore real-world degradations remains unexplored. Consequently, we extend our experiments to real restoration tasks using the real-world datasets SIDD~\citesupp{sidd} for denoising and RealSR~\citesupp{realsr} for super-resolution.

Specifically, SIDD~\citesupp{sidd} comprises images from 10 different static scenes captured using 5 different smartphone cameras. The dataset presents additional challenges for image denoising due to white noise and various camera settings, including lightness, brightness, and exposure. SIDD contains 320 training image pairs and 1,280 testing image pairs, which are cropped as patches from scenes not revealed in the training set. RealSR~\citesupp{realsr} includes 400 training image pairs and 100 testing image pairs, captured by two cameras: Canon 5D3 and Nikon D810, with various lens settings. The pairs are generated through sophisticated image registration operations. For more details about these datasets, please refer to their respective original papers.

We maintain the same training settings as described in the main manuscript for experiments on these datasets. The evaluation results are presented in Table~\ref{table::sidd_results} and Table~\ref{table::realsr_results}. Please note that PSNR/SSIM results in these two tables are computed on the Y channel from the YCbCr color space. In Table~\ref{table::sidd_results}, we observe that regardless of the training schemes applied to Restormer~\cite{restormer} or PromptIR~\cite{promptir}, the results are suboptimal. Furthermore, when trained with all four restoration tasks mentioned in the main manuscript, the performance of Restormer$_E$ and PromptIR$_E$ improves only marginally compared to the input low-quality images. However, when trained exclusively with synthetic noisy data, the performance gain is approximately 3 dB, which is a substantial improvement. In contrast, our proposed \modelname~outperforms other settings by a large margin. It is noteworthy that we select the middle checkpoint during the entire training process, and an improvement is achieved in just 5 hours, which demonstrates the effectiveness of our proposed method. In Table~\ref{table::realsr_results}, the significant domain gap between the pre-training data and downstream tasks appears larger as evidenced by the performance of Restormer$_E$ and PromptIR$_E$, which is even lower than the results of the bicubic interpolation method. Despite this, our method successfully adapts the foundation models Restormer$_E$ and Restormer-S$_E$ for the RealSR~\citesupp{realsr} with an upscaling factor of 4 in only 2 hours.

These observations illustrate that although there is a significant domain gap between synthetic and real datasets, \modelname~can effectively bridge this gap, extending the foundation model to real-world scenarios and proving the efficacy of our method.

\begin{figure*}[t]
    \centering
    \includegraphics[width=0.9\textwidth]{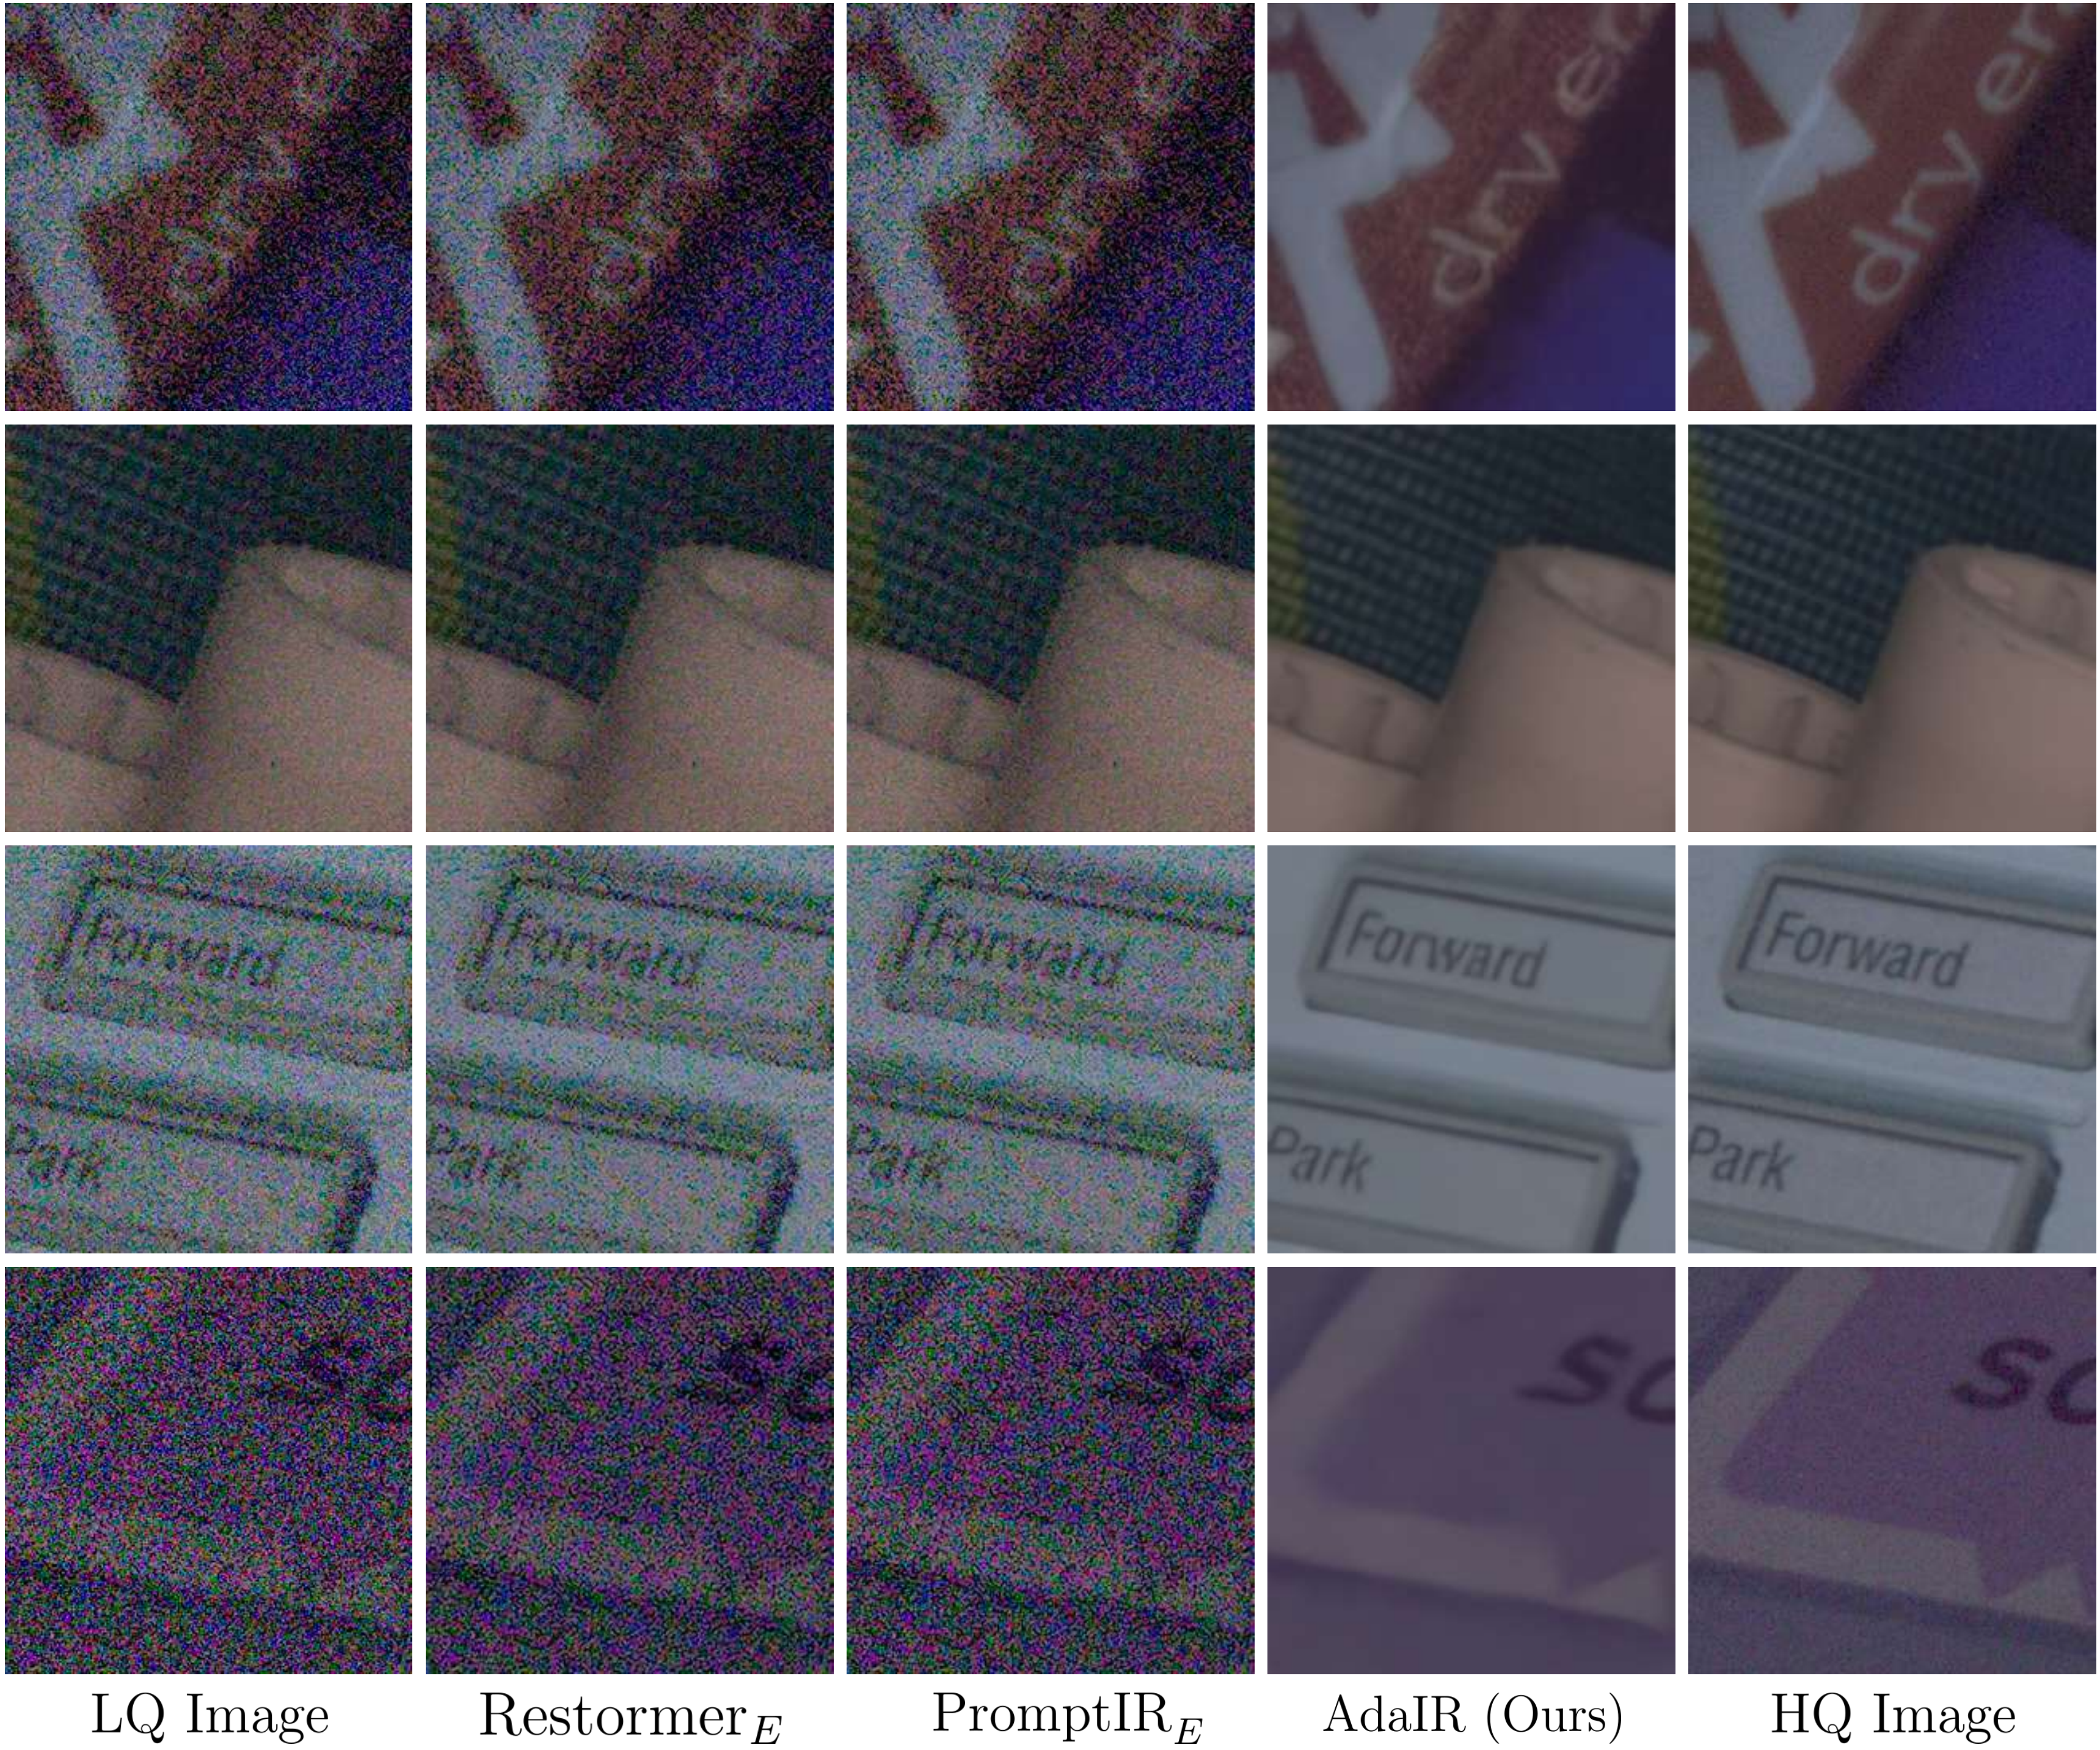}
    \caption{The qualitative results of $\text{Restormer}_{E+H}$, $\text{PromptIR}_{E+H}$, and our AdaIR in the real denoising task with using SIDD~\protect\citesupp{sidd} dataset.}
    \label{fig::qual_sidd}
\end{figure*}

\begin{figure*}[t]
    \centering
    \includegraphics[width=0.9\textwidth]{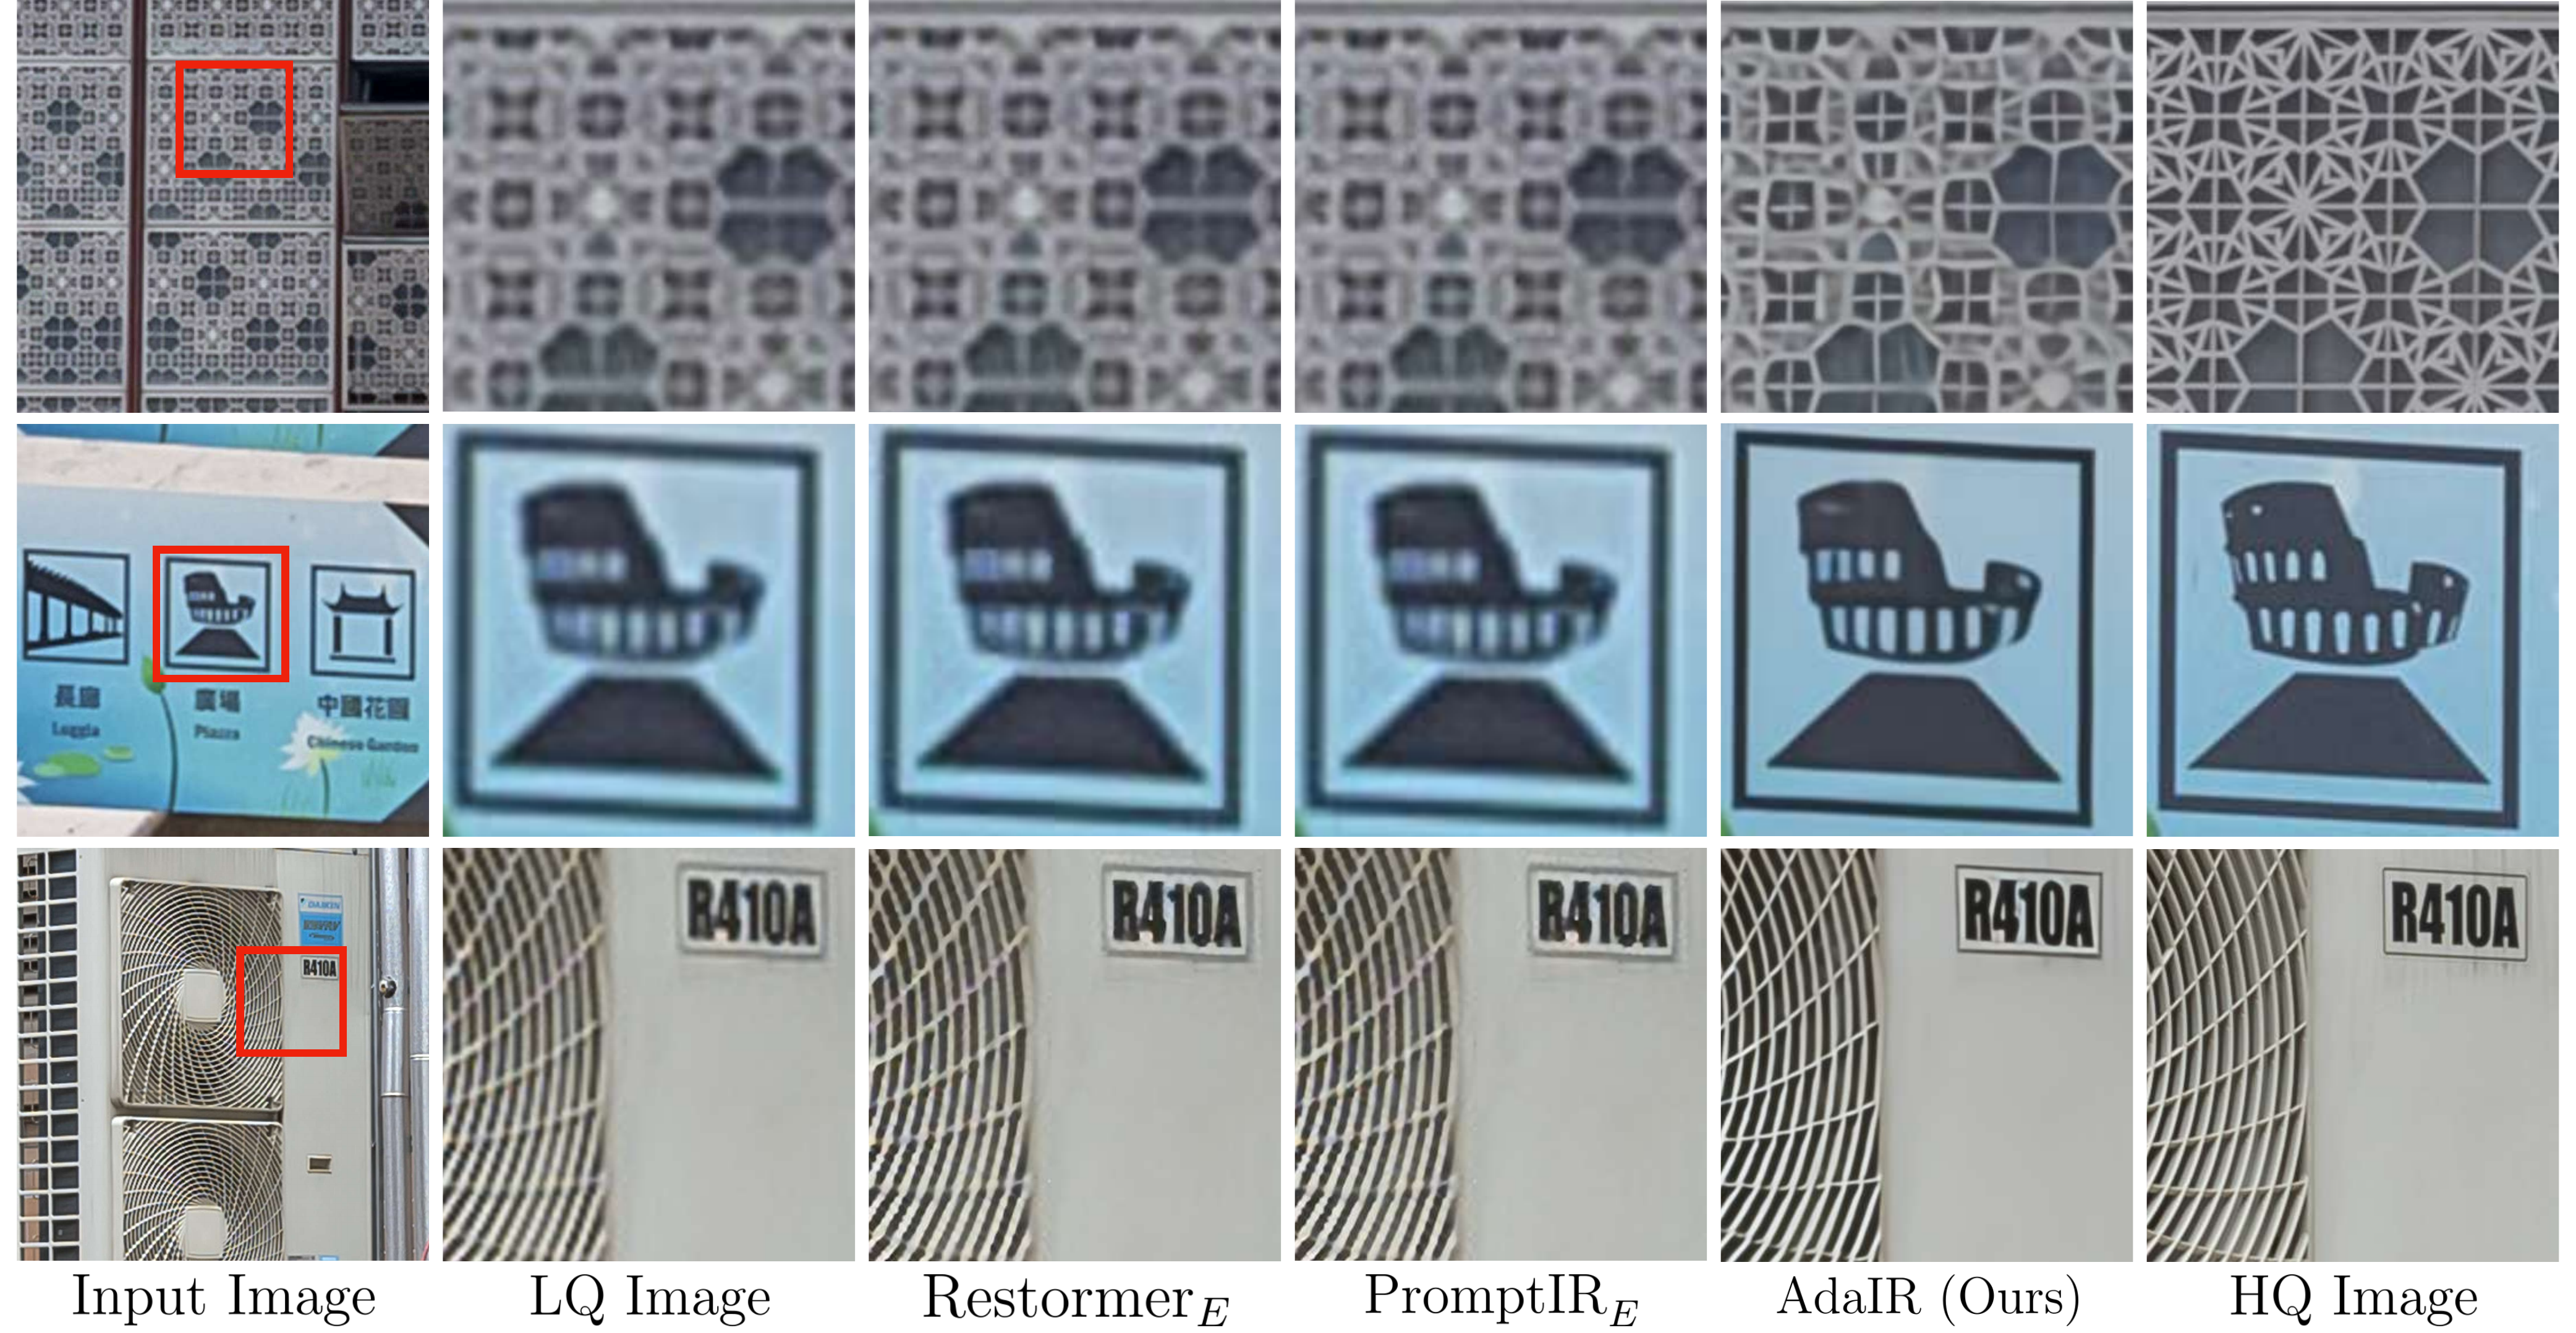}
    \caption{The qualitative results of $\text{Restormer}_{E+H}$, $\text{PromptIR}_{E+H}$, and our AdaIR in the super-resolution task with using RealSR~\protect\citesupp{realsr} dataset.}
    \label{fig::qual_realsr}
\end{figure*}

In addition to the quantitative results presented in Table~\ref{table::sidd_results} and Table~\ref{table::realsr_results}, we also provide qualitative results for the denoising and super-resolution tasks on real datasets, as illustrated in Fig.\ref{fig::qual_sidd} and Fig.\ref{fig::qual_realsr}. The qualitative outcomes corroborate the conclusions drawn from the quantitative data, which indicates that Restormer$_E$ and PromptIR$_E$ fail to produce satisfactory results from the input LQ images. In contrast, our method yields results that are more closely aligned with the HQ images. Notably, these results are achieved after only 2 hours for denoising and 5 hours for super-resolution tasks, respectively. In Fig.\ref{fig::qual_sidd}, while our method does not restore the noisy images to perfection and some artifacts remain, it successfully eliminates most of the noise present in the LQ images. In Fig.\ref{fig::qual_realsr}, the images reconstructed by our method exhibit sharp edges and clear patterns. For instance, in the first row, the cross patterns produced by Restormer$_E$ and PromptIR$_E$ appear blurry and discontinuous, whereas our results are coherent. In the third row, the 'R' character reconstructed by our method closely matches the HQ image.

%%%%%%%%% EXPERIMENTAL RESULTS
\subsection{Experimental Results}
\label{sec::supp_exp}

\subsubsection{SSIM Results.}
\begin{table}[t]
\centering
\footnotesize
\resizebox{\linewidth}{!}{
\begin{tabular}{l|P{10mm}P{12mm}|P{10mm}P{12mm}|P{10mm}P{10mm}|P{10mm}P{10mm}|P{10mm}P{10mm}|P{10mm}P{10mm}|P{20mm}}
\multirow{3}{*}{Method} & \multicolumn{4}{c|}{Gaussian Denoising}                      & \multicolumn{4}{c|}{Super-Resolution}                     & \multicolumn{4}{c|}{Gaussian Deblurring}                          & Deraining       \\ 
\cline{2-14}
                        & \multicolumn{2}{c|}{BSD68~\cite{bsd68}} & \multicolumn{2}{c|}{Urban100~\cite{urban100}} & \multicolumn{2}{c|}{B100~\cite{b100}} & \multicolumn{2}{c|}{Urban100~\cite{urban100}} & \multicolumn{2}{c|}{BSD68~\cite{bsd68}} & \multicolumn{2}{c|}{Urban100~\cite{urban100}} & Rain100H~\cite{rain100l} \\
                        & $\sigma=70$ & $\sigma=100$  & $\sigma=70$ & $\sigma=100$     & $\times 6$ & $\times 8$   & $\times 6$ & $\times 8$       & \textit{k19s4} & \textit{k21s5} & \textit{k19s4} & \textit{k21s5} & \textit{heavy}  \\ 
\specialrule{0.8pt}{0.0ex}{0.0ex}
Unet$_E$~\citesupp{unet}            & 0.413       & 0.210         & 0.487       & 0.276            & 0.518      & 0.541        & 0.545      & 0.496            & 0.589          & 0.541          & 0.553          & 0.497          & 0.540           \\
Restormer$_E$~\cite{restormer}      & 0.551       & 0.285         & 0.613       & 0.354            & 0.442      & 0.474        & 0.489      & 0.454            & 0.582          & 0.530          & 0.529          & 0.486          & 0.450           \\
PromptIR$_E$~\cite{promptir}        & 0.538       & 0.298         & 0.611       & 0.367            & 0.492      & 0.507        & 0.519      & 0.485            & 0.587          & 0.531          & 0.534          & 0.485          & 0.445           \\
Unet$_{E+H}$~\citesupp{unet}        & 0.749       & 0.691         & 0.823       & 0.773            & 0.647      & 0.596        & 0.671      & 0.544            & 0.738          & 0.687          & 0.757          & 0.688          & 0.899           \\
Restormer$_{E+H}$~\cite{restormer}  & \rb{0.756}       & \rb{0.698}         & \bu{0.836}       & \bu{0.790}            & \rb{0.655}      & \bu{0.605}        & \rb{0.697}      & \rb{0.614}            & \rb{0.758}          & \rb{0.717}          & \bu{0.797}          & \rb{0.744}          & \rb{0.921}           \\
PromptIR$_{E+H}$~\cite{promptir}    & \bu{0.753}       & 0.694         & \bu{0.836}       & \rb{0.791}            & \bu{0.654}      & \rb{0.606}        & \rb{0.697}      & 0.597            & \bu{0.754}          & 0.711          & \bu{0.797}          & \bu{0.741}          & \rb{0.921}           \\
AdaIR-UNet                              & 0.751       & 0.691         & 0.828       & 0.776            & 0.648            & 0.597             & 0.674           & 0.595                 & 0.751          & 0.690          & 0.775          & 0.698          & 0.883           \\
AdaIR                                   & \rb{0.756}       & \bu{0.697}         & \rb{0.838}       & \rb{0.791}            & \rb{0.655}      & 0.603        & \bu{0.694}      & \bu{0.606}           & \rb{0.758}          & \bu{0.713}          &  \rb{0.800}          & 0.740          & \bu{0.907}               
\end{tabular}
}
\caption{The average SSIM over the hard subsets of the restoration tasks including Gaussian denoising, super-resolution, Gaussian deblurring, and deraining. The best and second-best performing results are highlighted by the \rb{red} and \bu{blue} colors, respectively.}
\label{table::ssim_results}
\vspace{-10pt}
\end{table}

Table~\ref{table::ssim_results} presents the evaluation results for the hard subsets of four restoration tasks, measured in terms of Structural Similarity Index Measure (SSIM). The experimental settings include all configurations described in the main manuscript, in addition to the scenario where Unet~\citesupp{unet} serves as the foundation model. It is noteworthy that our proposed method, \modelname, achieves performances comparable to those of the baselines: Restormer$_{E+H}$ and PromptIR$_{E+H}$. Interestingly, when employing the Unet model as the foundation model, which comprises only 18.7 million parameters, approximately 70\% of the Restormer model's size, and lacks computationally intensive self-attention operations, it achieves results that are within 0.04 SSIM of the best setting.

\subsubsection{Single Task Training Results.}
\begin{table}[t]
\centering
\footnotesize
\resizebox{\linewidth}{!}{
\begin{tabular}{l|P{10mm}P{12mm}|P{10mm}P{12mm}|P{10mm}P{10mm}|P{10mm}P{10mm}|P{10mm}P{10mm}|P{10mm}P{10mm}}
\multirow{3}{*}{Method} & \multicolumn{4}{c|}{Gaussian Denoising}                      & \multicolumn{4}{c|}{Super-Resolution}                       & \multicolumn{4}{c}{Gaussian Deblurring}                            \\ 
\cline{2-13}
                        & \multicolumn{2}{c|}{BSD68~\cite{bsd68}} & \multicolumn{2}{c|}{Urban100~\cite{urban100}} & \multicolumn{2}{c|}{B100~\cite{b100}} & \multicolumn{2}{c|}{Urban100~\cite{urban100}} & \multicolumn{2}{c|}{BSD68~\cite{bsd68}}     & \multicolumn{2}{c}{Urban100~\cite{urban100}}    \\
                        & $\sigma=70$ & $\sigma=100$  & $\sigma=70$ & $\sigma=100$     & $\times 6$ & $\times 8$    & $\times 6$ & $\times 8$        & \textit{k19s4} & \textit{k21s5} & \textit{k19s4} & \textit{k21s5}  \\
\specialrule{0.8pt}{0.0ex}{0.0ex}
Restormer-S$_E$~\cite{restormer}        & 24.42       & 19.26         & 24.95       & 19.23            & 24.58      & 23.68         & 21.70      & 20.75             & 23.29          & 22.24          & 19.94          & 19.17           \\
PromptIR-S$_E$~\cite{promptir}          & 24.44       & 19.02         & 24.89       & 18.94            & 24.57      & 23.68         & 21.70      & 20.75             & 23.33          & 22.25          & 19.98          & 19.18           \\
Restormer-S$_{E+H}$~\cite{restormer}    & \rb{27.07}       & \rb{25.64}         & \rb{27.98}       & \rb{26.39}            & \rb{26.01}      & \rb{24.99}         & \rb{24.33}      & \bu{22.33}             & \bu{27.30}          & \rb{26.45}          & \bu{25.74}          & \bu{24.39}           \\
PromptIR-S$_{E+H}$~\cite{promptir}      & \bu{27.06}       & \bu{25.63}         & \bu{27.97}       & \bu{26.37}            & 25.84      & \rb{24.99}         & 23.91      & \rb{22.43}             & \rb{27.31}          & \bu{26.44}          & \rb{25.79}          & \rb{24.41}           \\
AdaIR-S                                     & 27.04       & 25.60         & 27.88       & 26.23            & \bu{25.92}      & \bu{24.85}         & \bu{24.10}      & 22.32             & 27.29          & 26.11          & 25.73          & 23.90          
\end{tabular}
}
\caption{The average PSNR (dB) over the hard subsets of the restoration tasks including Gaussian denoising, super-resolution, and Gaussian deblurring. The best and second-best performing results are highlighted by the \rb{red} and \bu{blue} colors, respectively.}
\label{table::single_task_results}
\vspace{-10pt}
\end{table}
In the main manuscript, we primarily present results from experimental settings where foundation models are trained using the subsets of all restoration tasks. In this section, we offer additional experiments where the models are trained exclusively on a specific restoration task. Table~\ref{table::single_task_results} compares our proposed method with others within the single-task domain. Theoretically, this single-task setting should yield the best performance for each restoration task, as the model can focus solely on the target task without being influenced by other restoration tasks or different types of degradations.

However, our study is centered on the integration of lightweight adapter modules into the foundation model to address multiple degradations. Consequently, while the single-task setting may achieve optimal performance for each individual task, these results are not included in the main manuscript due to our broader focus. Notwithstanding, it is noteworthy that in Table~\ref{table::single_task_results}, our proposed method AdaIR-S still manages to achieve comparable results against Restormer-S$_{E+H}$ and PromptIR-S$_{E+H}$, in Gaussian denoising, super-resolution, and Gaussian deblurring tasks.

\subsubsection{Easy Setting Results.}
\begin{table}[t]
\centering
\footnotesize
\resizebox{\linewidth}{!}{
\begin{tabular}{l|P{10mm}P{10mm}P{10mm}|P{10mm}P{10mm}P{10mm}|P{10mm}P{10mm}P{10mm}|P{10mm}P{10mm}P{10mm}|P{20mm}}
\multirow{3}{*}{Method} & \multicolumn{6}{c|}{Gaussian Denoising}                                                                                     & \multicolumn{6}{c|}{Gaussian Deblurring}                                                                                                     & Deraining       \\ 
\cline{2-14}
                        & \multicolumn{3}{c|}{BSD68~\cite{bsd68}} & \multicolumn{3}{c|}{Urban100~\cite{urban100}} & \multicolumn{3}{c|}{BSD68~\cite{bsd68}} & \multicolumn{3}{c|}{Urban100~\cite{urban100}} & Rain100L~\cite{rain100l}        \\
                        & $\sigma=15$ & $\sigma=25$ & \multicolumn{1}{l|}{$\sigma=50$} & $\sigma=15$ & $\sigma=25$ & \multicolumn{1}{l|}{$\sigma=50$} & \textit{k7s1} & \textit{k11s2} & \multicolumn{1}{l|}{\textit{k15s3}} & \textit{k7s1} & \textit{k11s2} & \multicolumn{1}{l|}{\textit{k15s3}} & \textit{light}  \\ 
\specialrule{0.8pt}{0.0ex}{0.0ex}
Unet$_E$~\citesupp{unet}            & 34.14       & 31.49       & 28.22                            & 33.89       & 31.67       & 28.57                            & 37.53         & 30.29          & 28.19                               & 35.10         & 28.45          & 26.27                               & 38.08           \\
Restormer$_E$~\cite{restormer}      & \bu{34.28}       & \bu{31.63}       & \bu{28.38}                            & \bu{34.31}       & \bu{32.09}       & \bu{29.03}                            & \bu{38.17}         & \rb{30.59}          & \rb{28.44}                               & \rb{36.22}         & \rb{29.61}          & \rb{27.19}                               & 38.27           \\
PromptIR$_E$~\cite{promptir}        & \rb{34.29}       & \rb{31.64}       & \rb{28.39}                            & \rb{34.32}       & \rb{32.10}       & \rb{29.05}                            & 37.79         & \bu{30.55}          & \bu{28.40}                               & 35.11         & \bu{29.45}          & 27.06                               & 38.15           \\
Unet$_{E+H}$ ~\citesupp{unet}       & 34.07       & 31.43       & 28.22                            & 33.71       & 31.54       & 28.51                            & 36.26         & 29.62          & 27.84                               & 32.68         & 27.16          & 25.50                               & 38.42           \\
Restormer$_{E+H}$~\cite{restormer}  & 34.26       & 31.61       & \rb{28.39}                            & 34.20       & 32.00       & 29.01                            & 37.96         & 30.38          & 28.39                               & \bu{36.05}         & 29.01          & 27.08                               & \bu{39.67}           \\
PromptIR$_{E+H}$~\cite{promptir}    & 34.26       & 31.61       & 28.37                            & 34.18       & 31.99       & 28.99                            & \rb{38.21}         & 30.36          & \bu{28.40}                               & 35.89         & 29.09          & \bu{27.16}                               & \rb{39.64}          
\end{tabular}
}
\caption{The average PSNR (dB) over the easy subsets of the restoration tasks including Gaussian denoising, Gaussian deblurring, and deraining. The best and second-best performing results are highlighted by the \rb{red} and \bu{blue} colors, respectively.}
\label{table::easy_results}
\vspace{-15pt}
\end{table}

\begin{table}[t]
\centering
\footnotesize
\resizebox{\linewidth}{!}{
\begin{tabular}{l|P{10mm}P{10mm}P{10mm}|P{10mm}P{10mm}P{10mm}|P{10mm}P{10mm}P{10mm}|P{10mm}P{10mm}P{10mm}}
\multirow{2}{*}{Method} & \multicolumn{3}{c|}{Set5~\cite{set5}} & \multicolumn{3}{c|}{Set14~\cite{set14}} & \multicolumn{3}{c|}{B100~\cite{b100}} & \multicolumn{3}{c}{Urban100~\cite{urban100}} \\
                        & $\times 2$ & $\times 3$ & $\times 4$ & $\times 2$ & $\times 3$ & $\times 4$ & $\times 2$ & $\times 3$ & $\times 4$ & $\times 2$ & $\times 3$ & $\times 4$  \\ 
\specialrule{0.8pt}{0.0ex}{0.0ex}
Bicubic                             & 33.66      & 30.39      & 28.42                           & 30.24      & 27.55      & 26.00      & 29.56      & 27.21      & 25.96      & 26.88      & 24.46      & 23.14       \\ 
\specialrule{0.8pt}{0.0ex}{0.0ex}
Unet$_E$~\citesupp{unet}            & 37.32      & 33.33      & 31.81                           & 33.10      & 29.84      & 28.40      & 32.02      & 28.65      & 27.50      & 31.17      & 27.62      & 25.74       \\
Restormer$_E$~\cite{restormer}      & \rb{38.08}      & \rb{34.66}      & \rb{32.51}                           & \bu{33.67}      & \bu{30.53}      & \rb{28.81}      & \rb{32.24}      & \bu{29.24}      & \rb{27.70}      & \rb{32.31}      & \rb{28.62}      & \rb{26.50}       \\
PromptIR$_E$ ~\cite{promptir}   & \rb{38.08}      & \bu{34.64}      & \bu{32.47}                           & \rb{33.71}      & \rb{30.54}      & \bu{28.79}      & \bu{32.23}      & \rb{29.25}      & \rb{27.70}      & \bu{32.27}      & \bu{28.60}      & \bu{26.48}       \\
Unet$_{E+H}$~\citesupp{unet}        & 37.07      & 32.54      & 31.35                           & 32.74      & 29.54      & 28.22      & 31.92      & 28.48      & 27.47      & 30.75      & 27.15      & 25.53       \\
Restormer$_{E+H}$~\cite{restormer}  & 37.92      & 34.50      & 32.42                           & 33.40      & 30.43      & 28.73      & 32.14      & 29.18      & 27.68      & 31.89      & 28.40      & 26.39       \\
PromptIR$_{E+H}$~\cite{promptir}    & \bu{37.95}      & 34.56      & \rb{32.51}                           & 33.53      & 30.44      & 28.78      & 32.18      & 29.20      & \bu{27.69}      & 31.99      & 28.47      & 26.46      
\end{tabular}
}
\caption{The average PSNR (dB) on Set5~\cite{set5}, Set14~\cite{set14}, B100~\cite{b100}, and Urban100~\cite{urban100} of super-resolution with scaling factor $\times 2$, $\times 3$, and $\times 4$. The best and second-best performing results are highlighted by the \rb{red} and \bu{blue} colors, respectively.}
\label{table::easy_sr_results}
\vspace{-15pt}
\end{table}

Previous tables, including those in the main manuscript and supplementary materials, focus on evaluating the performance of methods on the hard subsets of restoration tasks. However, the performance of these methods on the easy subsets has not been addressed. To fill this gap, Table~\ref{table::easy_results} and Table~\ref{table::easy_sr_results} present the evaluation results of these methods on the easy subsets of restoration tasks, measured in terms of PSNR.

In Table~\ref{table::easy_results}, we show the evaluation results for the easy subsets of Gaussian denoising, Gaussian deblurring, and deraining tasks. With the exception of the deraining task, it is observed that methods trained solely on easy subsets generally achieve better outcomes compared to those trained on both easy and hard subsets. This finding suggests that the models still treat each level of degradation as a distinct task, even when the types of degradation are identical. Consequently, when these models are trained with a broader range of restoration pairs, their capacity is dispersed, leading to suboptimal results on specific tasks but overall strong performance across all tasks.

An exception is observed in the deraining task, where the best performance is achieved when training includes the hard subsets. In conjunction with the evaluation results for the hard subsets of the deraining task in Table 1 of the main manuscript, we note that models trained with the hard subset of the deraining task perform well on both easy and hard subsets. In contrast, models trained only on the easy subset excel on the easy subset but falter on the hard subset. This discrepancy arises because the hard subset encompasses the easy subset, whereas the reverse is not true.

It is also worth mentioning that the results for the Gaussian deblurring task are inconsistent. This variability may stem from the design of the blurring kernel generation pipeline. The standard deviation $s$ in the blurring kernels is sampled from a uniform distribution, which tends to result in most sampled values clustering around the midpoint of the distribution range. For instance, with a uniform distribution $s \sim \mathcal{U}(3.0, 5.0)$, the sampled standard deviation is likely to be close to 4, rather than 3 or 5. If the testing set is defined with a standard deviation of 4, the model may overfit to this configuration and perform inconsistently when the standard deviation deviates from 4.

\begin{figure*}[t]
    \centering
    \includegraphics[width=0.9\textwidth]{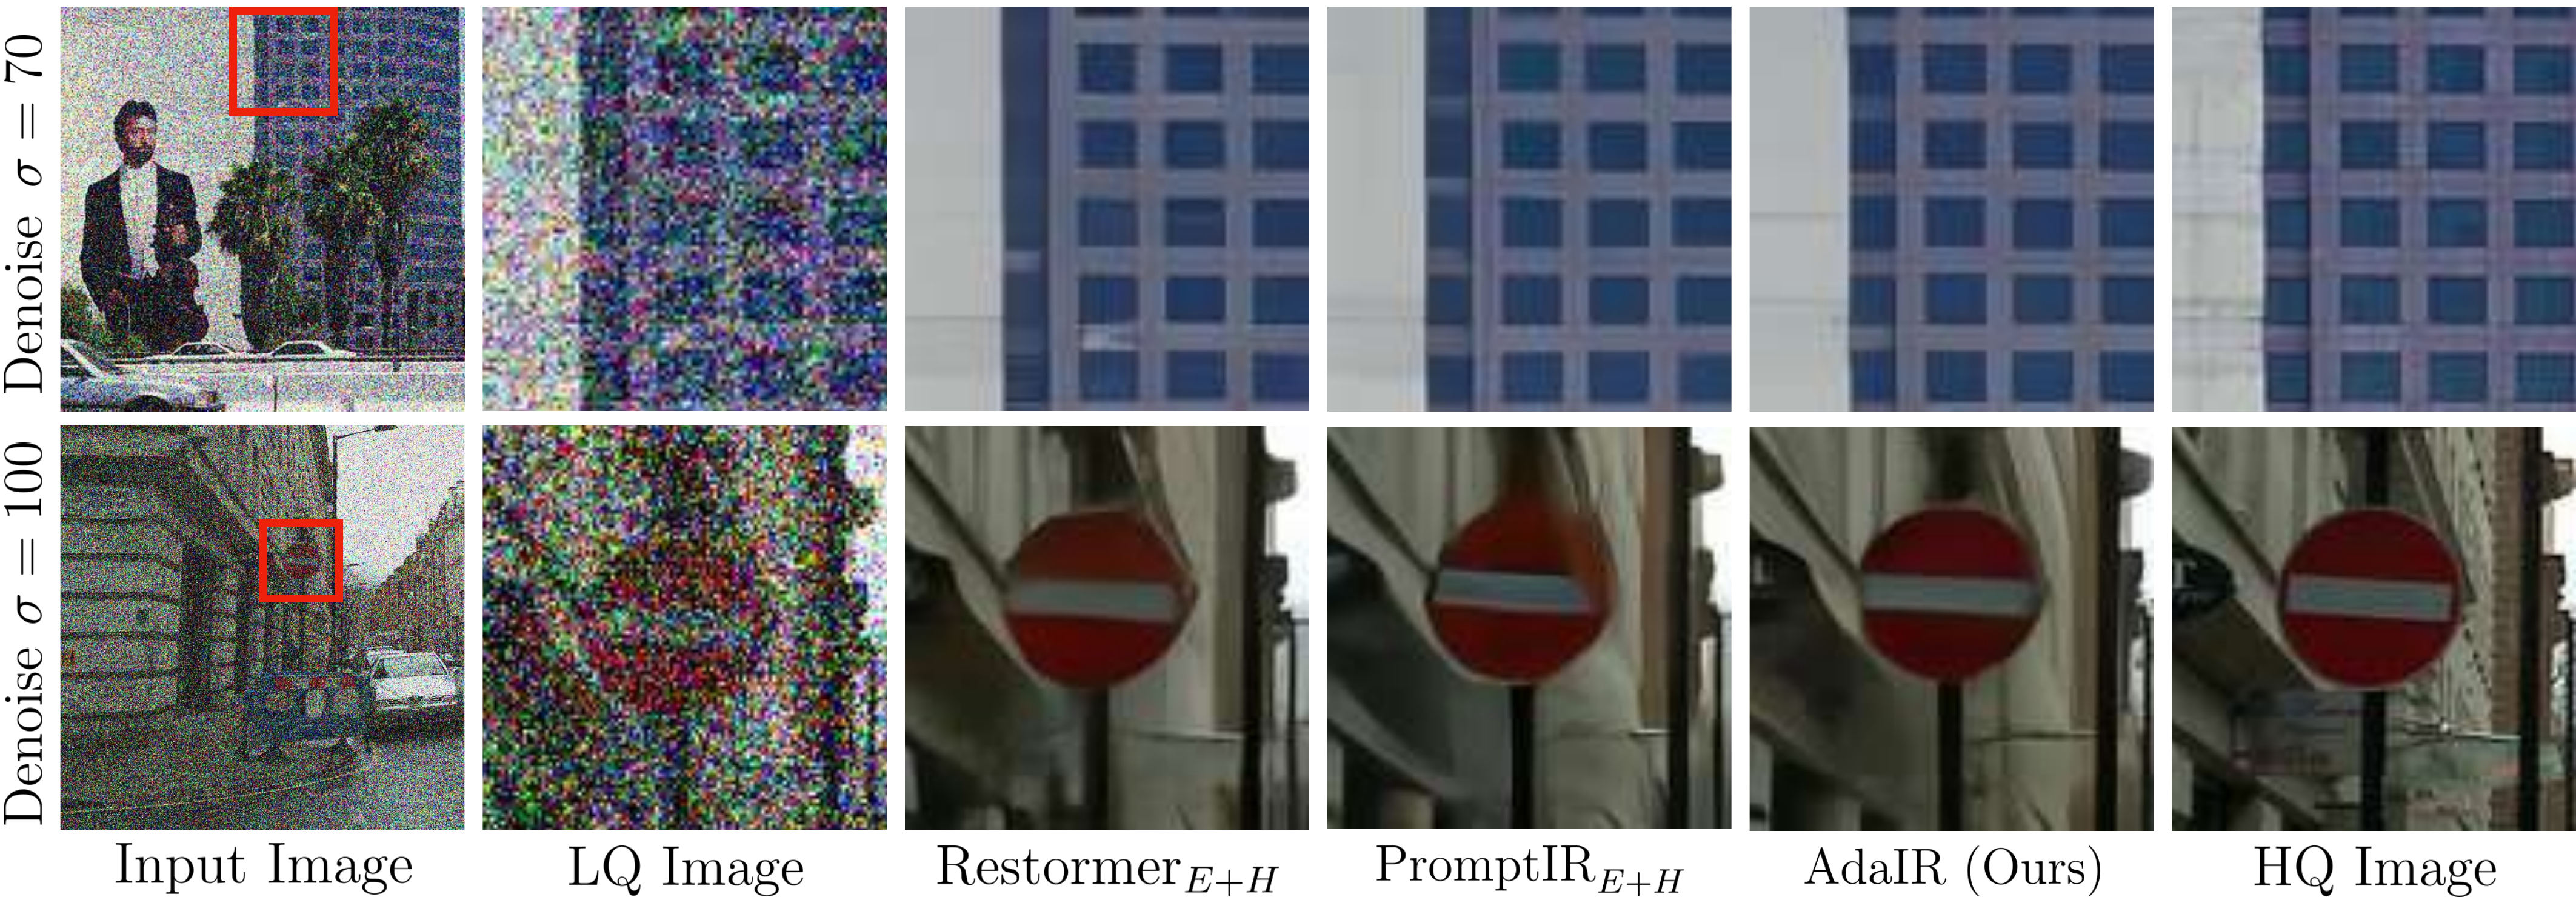}
    \caption{The qualitative results of $\text{Restormer}_{E+H}$, $\text{PromptIR}_{E+H}$, and our AdaIR in the denoising task with two noisy levels, and BSD68~\cite{bsd68} and Urban100~\cite{urban100} datasets are used.}
    \label{fig::qual_supp_denoise}
    \vspace{-10pt}
\end{figure*}

\begin{figure*}[t]
    \centering
    \includegraphics[width=0.9\textwidth]{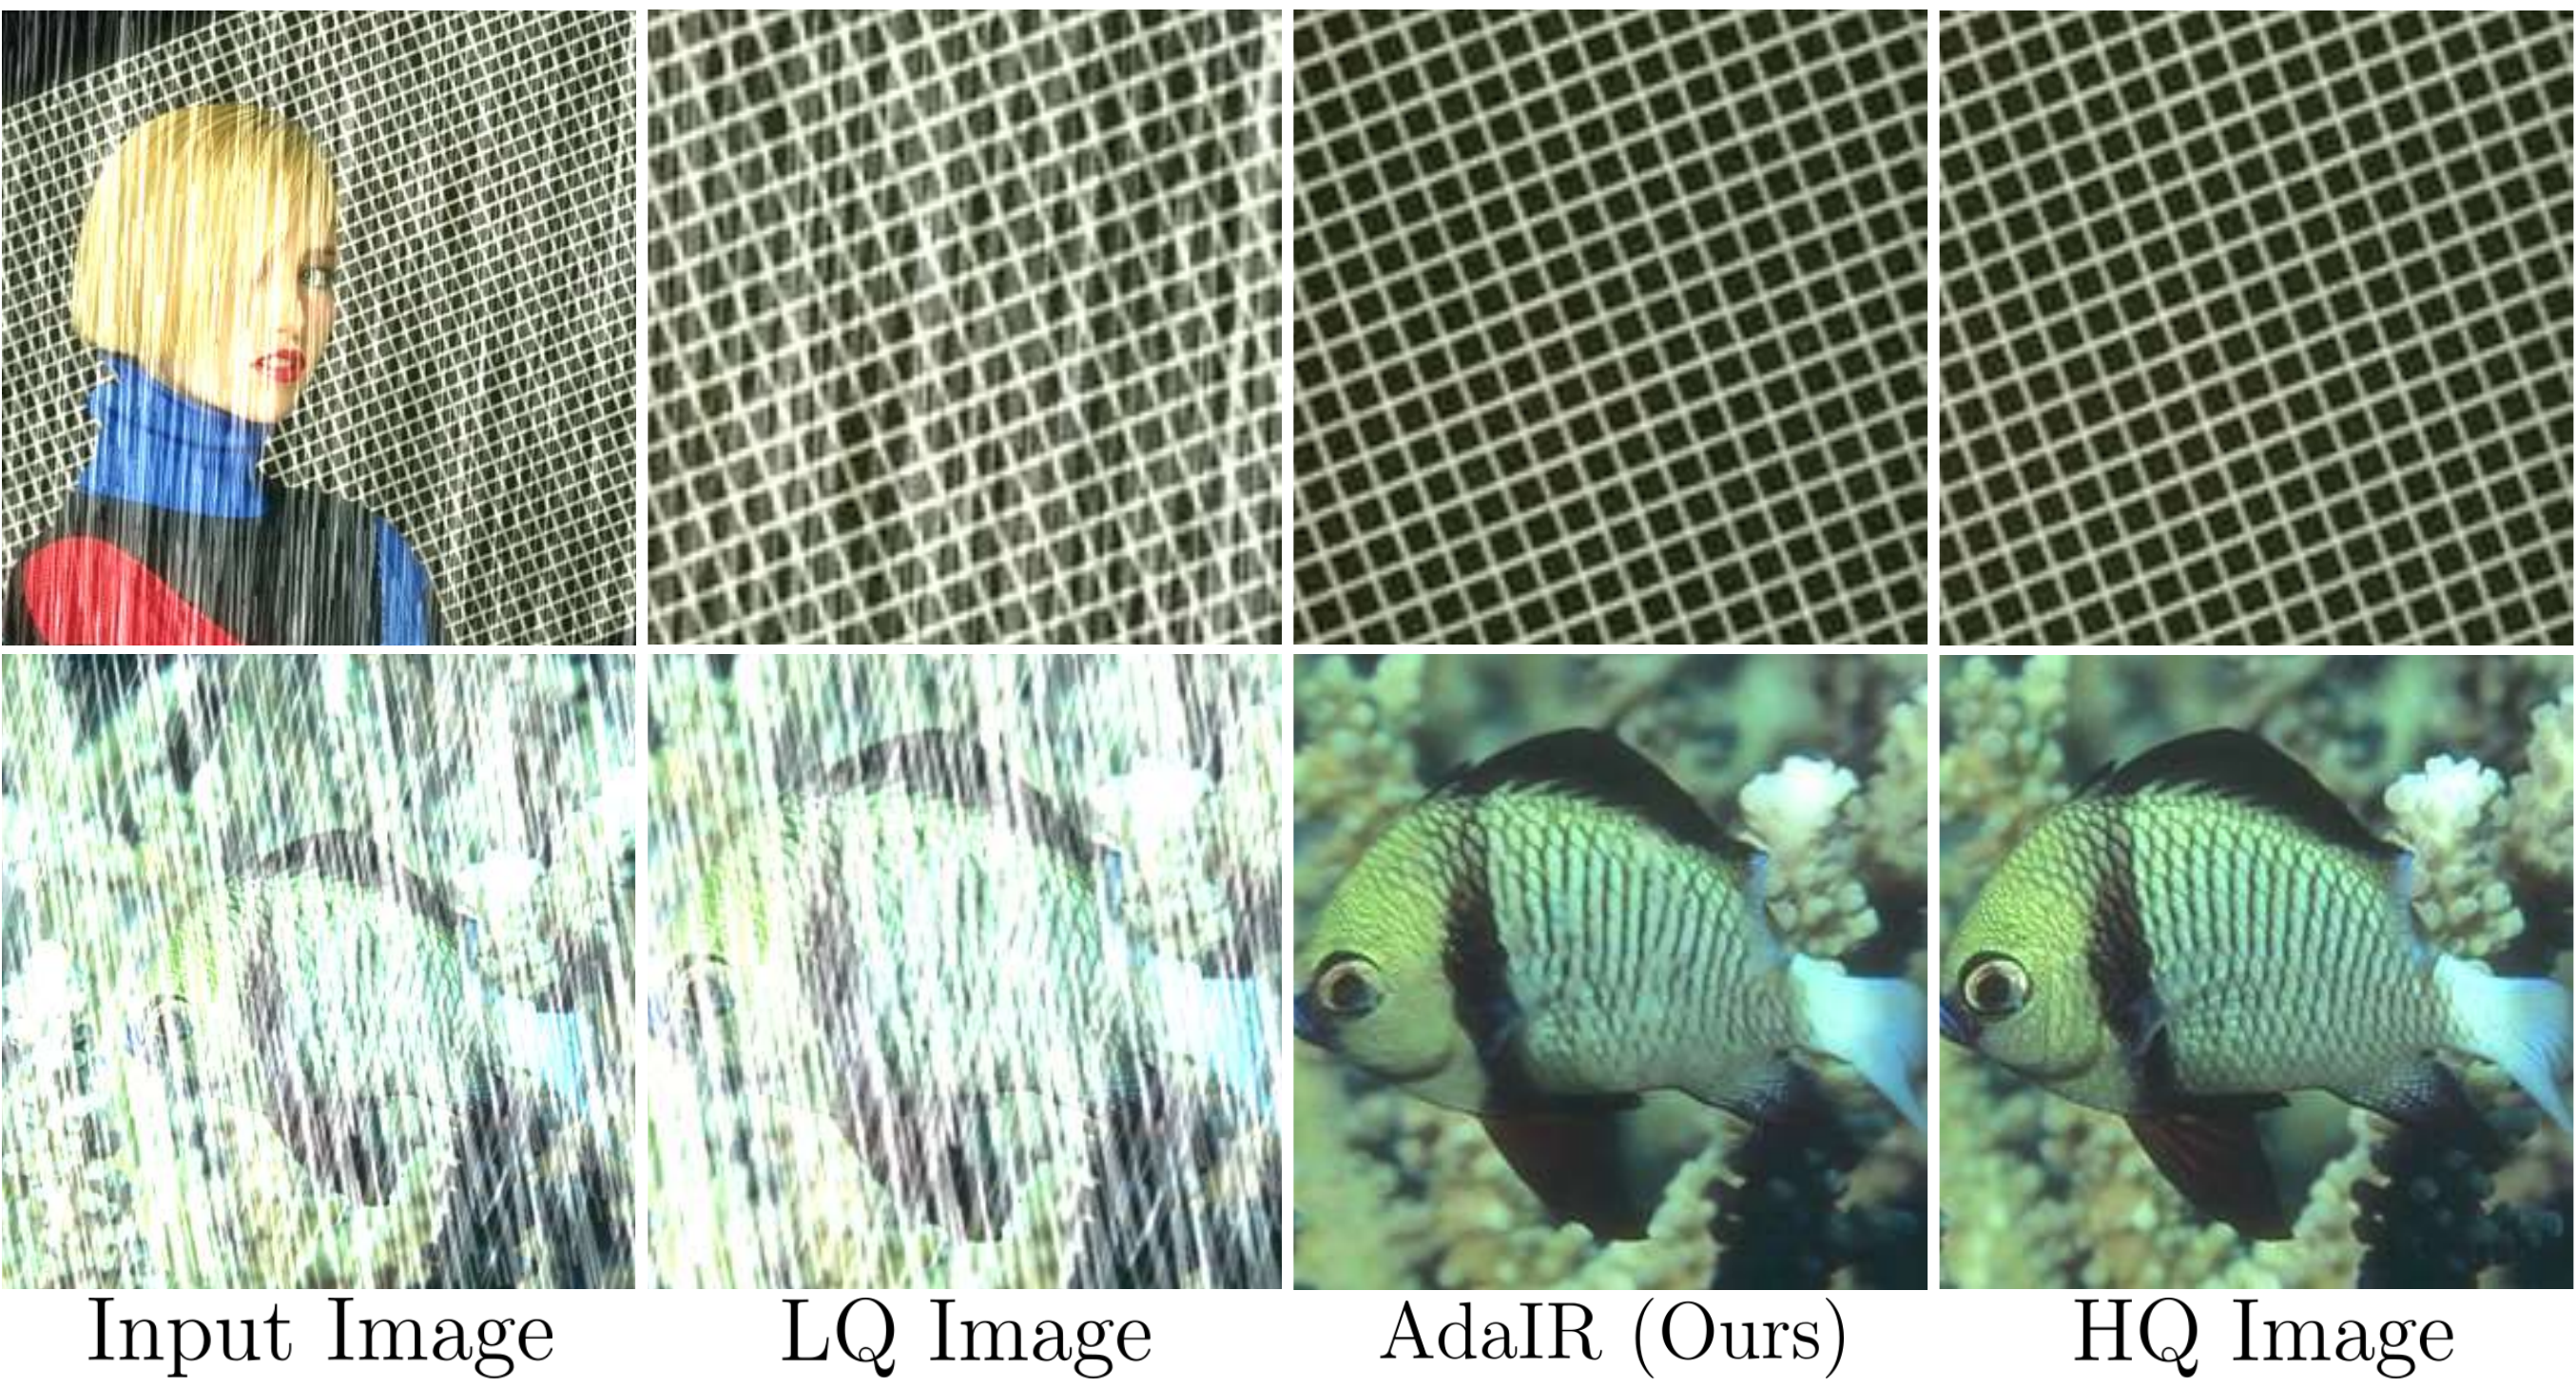}
    \caption{The qualitative results of our AdaIR in the draining task.}
    \label{fig::qual_supp_derain}
    \vspace{-10pt}
\end{figure*}

\begin{figure*}[t]
    \centering
    \includegraphics[width=0.9\textwidth]{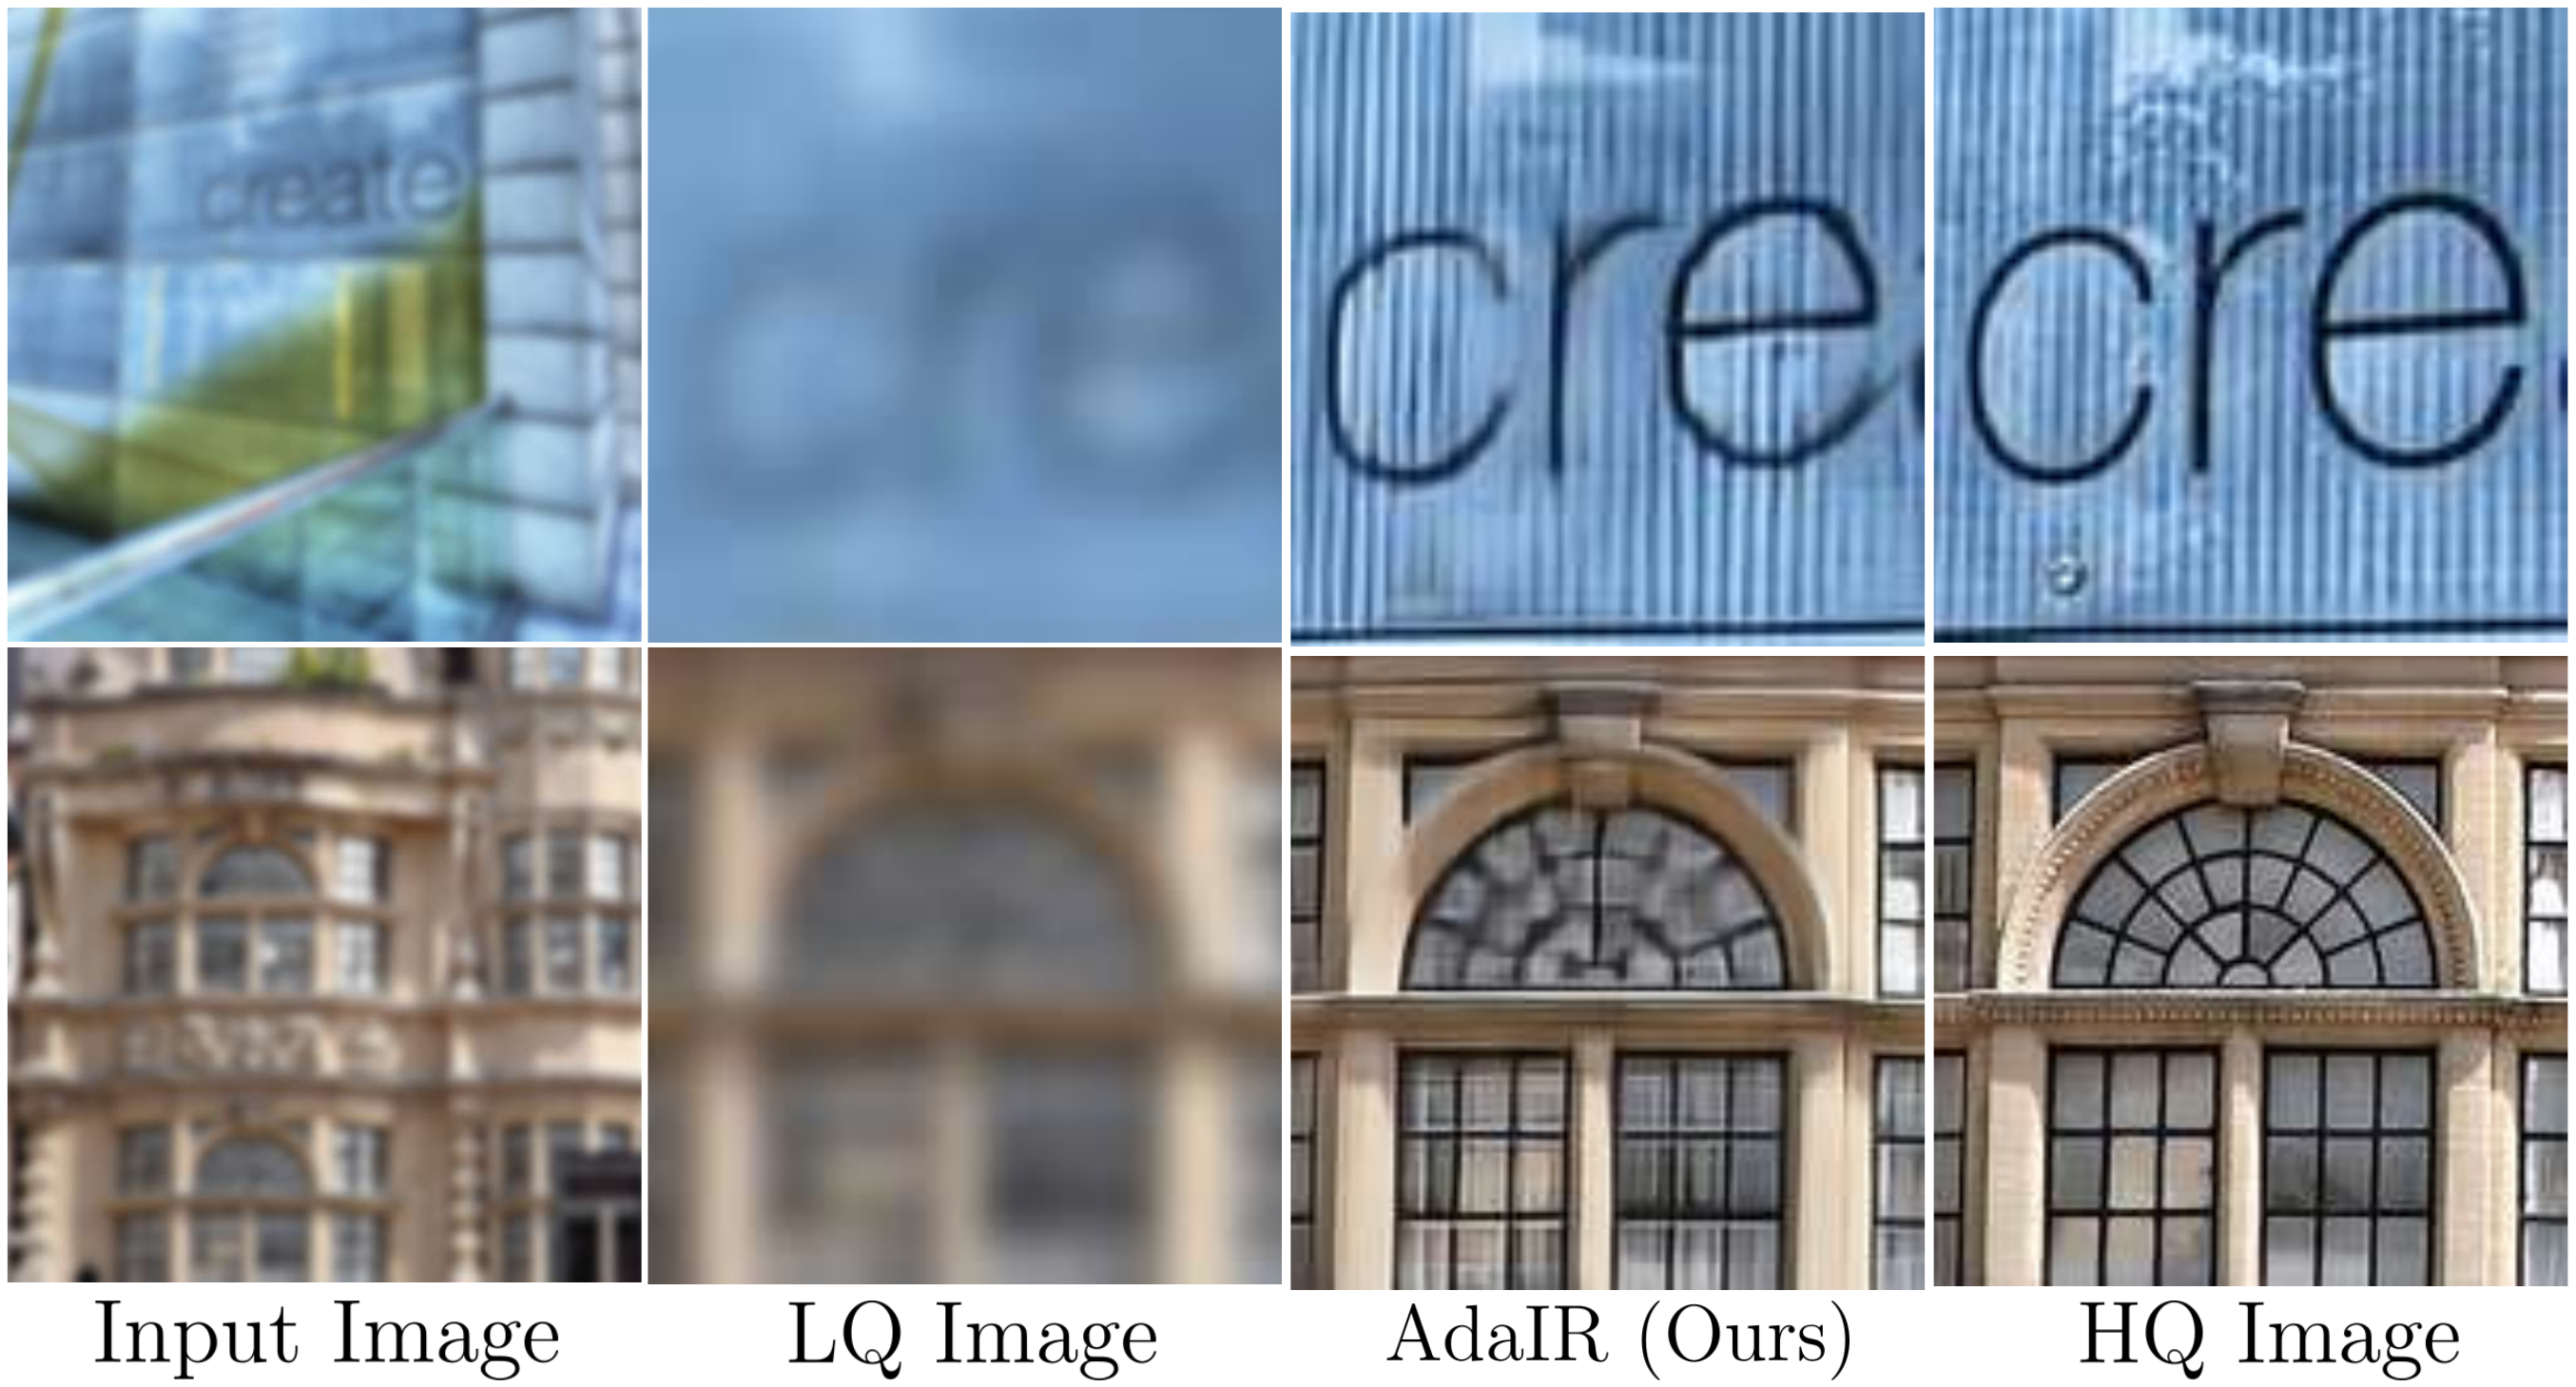}
    \caption{The qualitative results of our AdaIR in the Gaussian deblurring task, and the $k21s5$ configuration are used.}
    \label{fig::qual_supp_gd}
    \vspace{-20pt}
\end{figure*}

\begin{figure*}[t]
    \centering
    \includegraphics[width=0.9\textwidth]{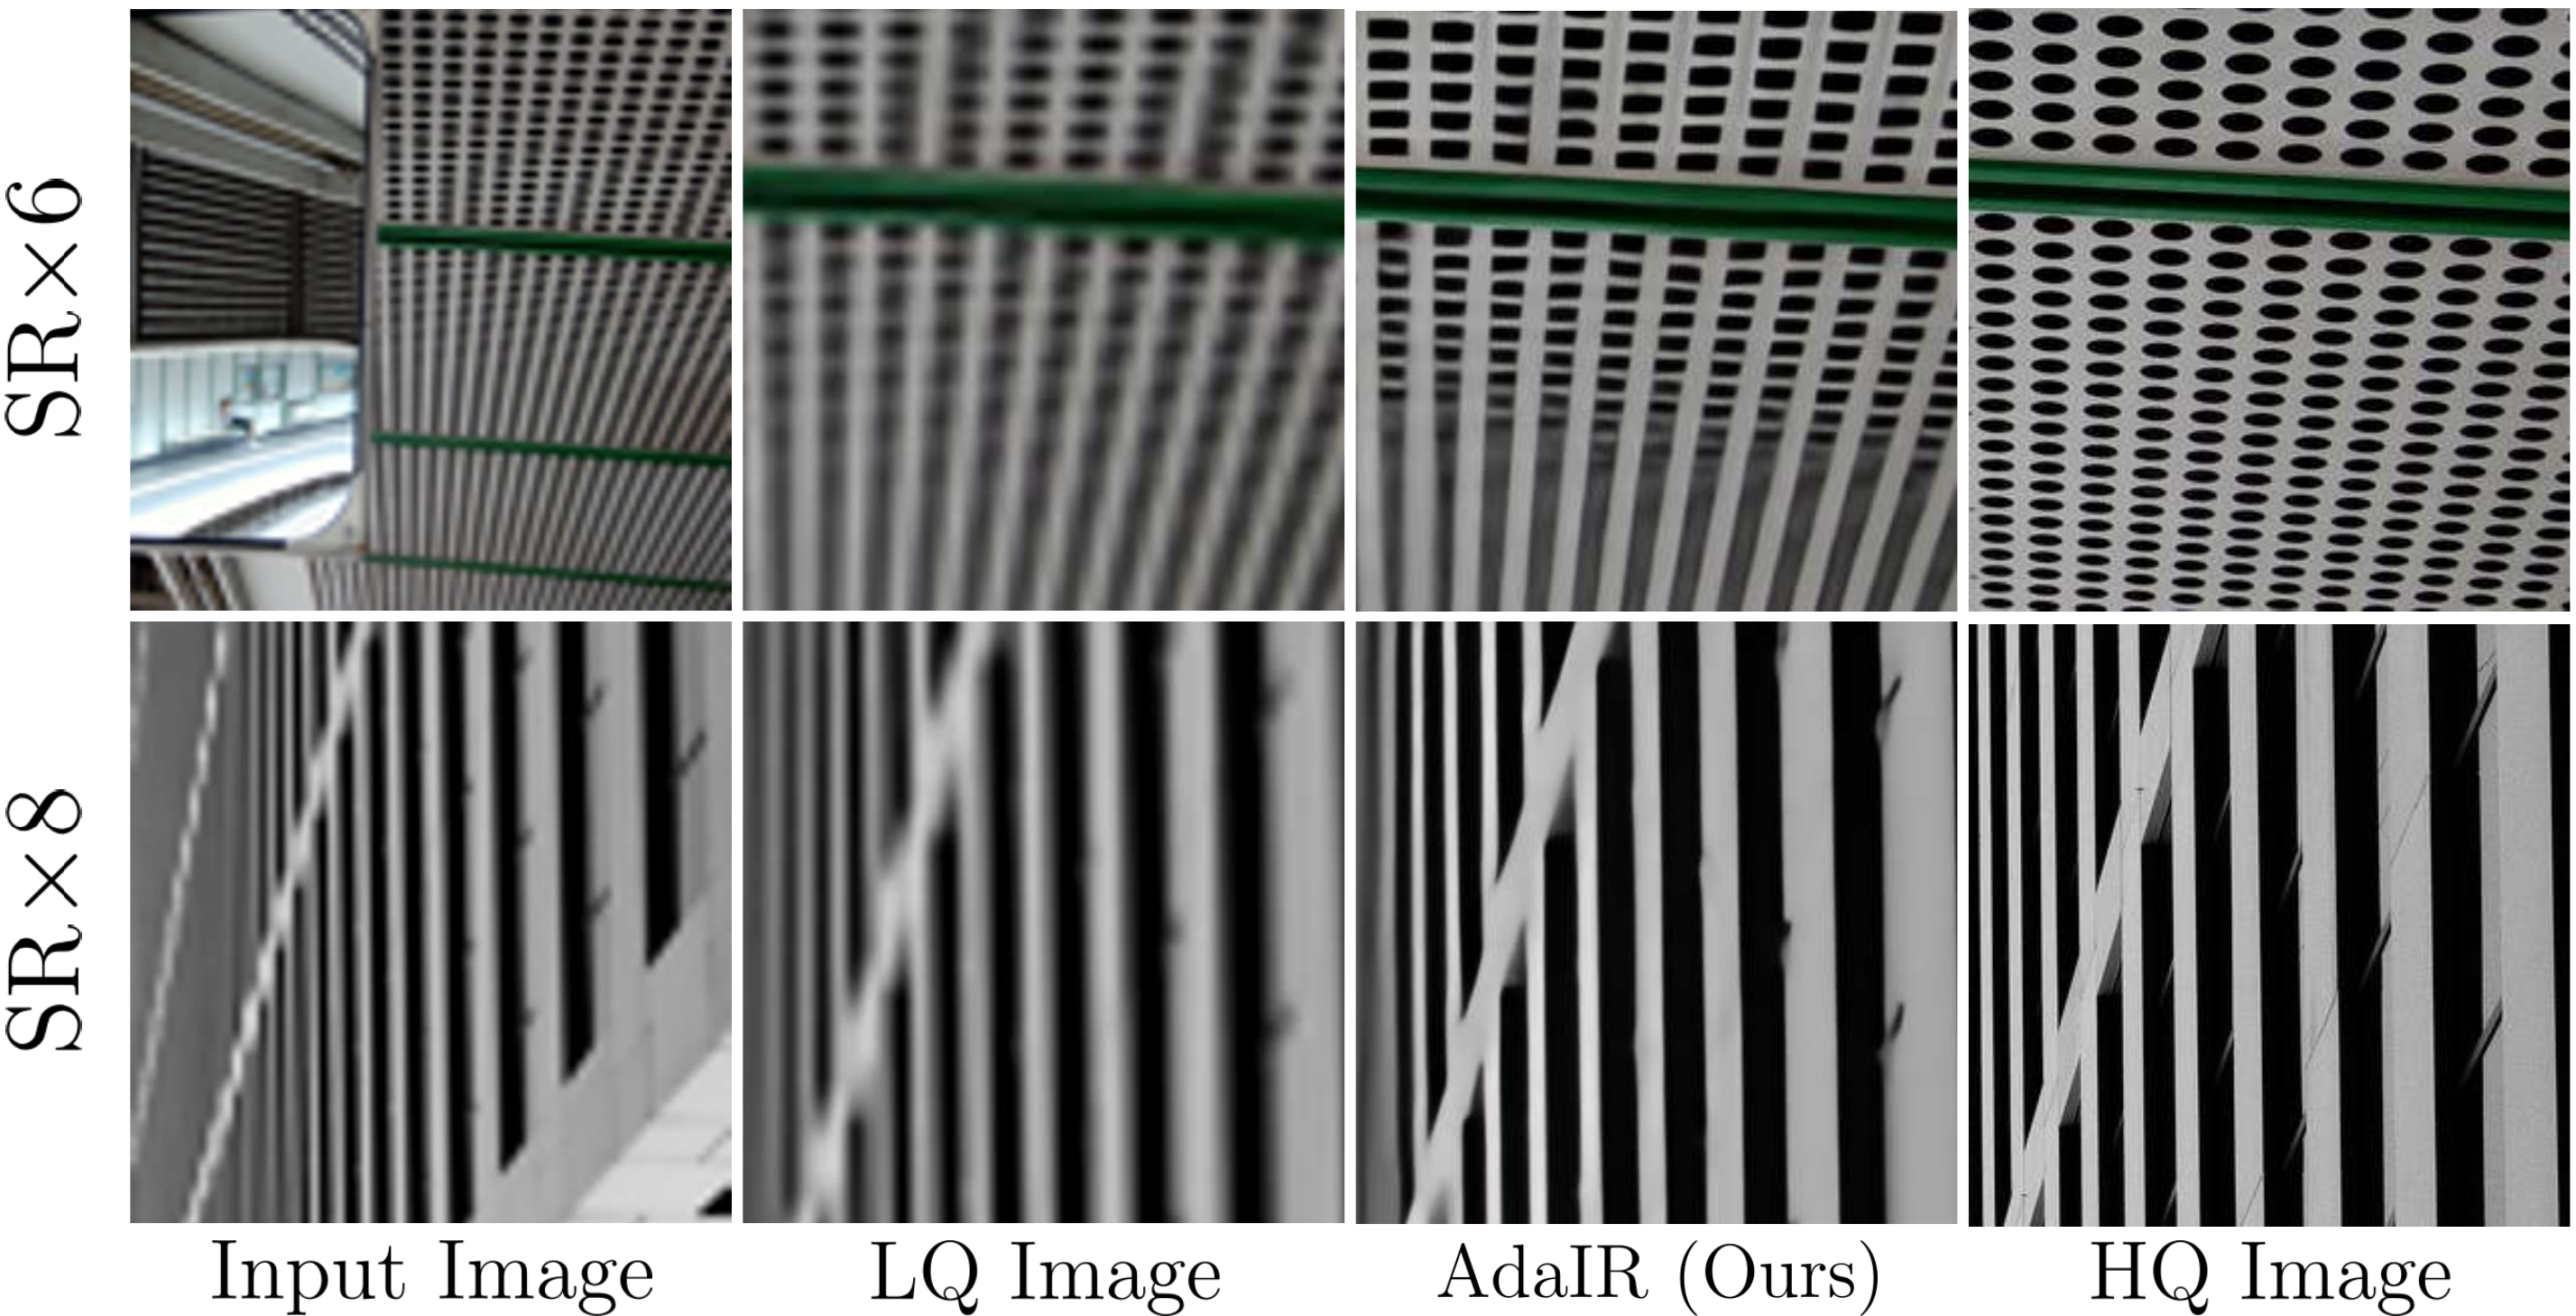}
    \caption{The qualitative results of our AdaIR in the super-resolution task, and two upscaling factors of 6 and 8 are involved in the illustration.}
    \label{fig::qual_supp_sr}
    \vspace{-20pt}
\end{figure*}

\subsubsection{Qualitative Results.}
In this section, we present additional qualitative results of our proposed method and compare them with baseline models. Fig.\ref{fig::qual_supp_denoise} displays the qualitative results of the proposed \modelname, Restormer$_{E+H}$ and PromptIR$_{E+H}$ on two benchmark denoising datasets: BSD68\cite{bsd68} and Urban100~\cite{urban100}. The noise levels $\sigma$ of the input images are set to 70 and 100, respectively. The first row demonstrates that, aside from our method, the other baseline models produce results with discontinuous and unclear building walls. The second row reveals that the stop sign reconstructed by our method closely resembles the HQ image, in contrast to the less accurate results from the other two baseline methods.
Fig.~\ref{fig::qual_supp_derain} presents the qualitative results of our method on the deraining task. In these two examples, we observe that our method can accurately restore LQ images, even when rain streaks are superimposed over white background patterns. Remarkably, in the second row, despite the fish scales being obscured by rain streaks, our method is still able to partially reconstruct them.
Fig.~\ref{fig::qual_supp_gd} showcases the qualitative results of our method on the Gaussian deblurring task, employing the $k21s5$ configuration. In the first row, the three alphabets, which are nearly unrecognizable in the LQ image, are reconstructed by our method into a clear form. In the second row, although some artifacts are present, our method successfully restores the window pattern, which is significantly degraded in the LQ image.
Fig.~\ref{fig::qual_supp_sr} illustrates the qualitative results of our method on the SR task with two upscaling factors, 6 and 8. These examples, while challenging, demonstrate that our method can capture and restore some patterns, despite the presence of artifacts and the significant difference between the LQ and HQ images. This further validates the effectiveness of our proposed \modelname.

%%%%%%%%% LIMITATIONS
\subsection{Limitations}
\label{sec::supp_limitations}
In this section, we discuss the limitations of our proposed method, \modelname, and outline potential future research directions. While our method achieves results comparable to the baseline models  Restormer$_E$ and PromptIR$_{E}$ in Gaussian denoising, Gaussian deblurring, and super-resolution tasks, there remains a noticeable performance gap in the deraining task. We hypothesize that this shortfall is due to the foundation model's inability to learn an effective feature extraction mechanism for addressing the hard subset of the deraining task during the pre-training phase. Since the foundation model is frozen and only the parameters within the adapter modules are adjustable, these limited parameters may be insufficient to capture the necessary features for robust heavy rain streak removal.

Beyond the suboptimal results in the deraining task, we have not identified a universally optimal pre-training scheme for the foundation model to adapt to the various restoration tasks discussed previously. For instance, pre-training the foundation model with noisy data pairs proves most effective for the denoising task, whereas pre-training with all types of degradation is most beneficial for the Gaussian deblurring task. Consequently, determining the most favorable pre-training scheme for the foundation model is an important direction for future research. We hope that the analysis and experimental results presented in this paper will contribute to broader developments and research in this field.

%%%%%%%%% CITATIONS
\bibliographystylesupp{splncs04}
\bibliographysupp{citations}
