# Supplementary material for: AdaIR: Exploiting Underlying Similarities of Image Restoration Tasks with Adapters
Source: arXiv:2404.11475 source file (2024-04-17)
Supplement: Supplementary file 2 [file a0.supp.tex]

\section{Supplementary Material}
\label{sec::supp_material}
This supplementary material is organized as follows.
Section~\ref{sec::supp_unet} demonstrates the flexibility of the foundation model in our \modelname~framework.
Section~\ref{sec::supp_real} presents additional results on real datasets. Section~\ref{sec::supp_exp} provides further experimental results of \modelname~. Finally, the limitations of our proposed \modelname~are summarized in Section~\ref{sec::supp_limitations}.
