# Supplementary material for: AdaIR: Exploiting Underlying Similarities of Image Restoration Tasks with Adapters
Source: arXiv:2404.11475 source file (2024-04-17)
Supplement: Supplementary file 6 [file notations.tex]

\begin{table}[ht]
\centering
\footnotesize
\resizebox{\linewidth}{!}{
\begin{tabular}{l|l} 
\specialrule{0.8pt}{0.0ex}{0.0ex}
\textbf{Symbol}     & \textbf{Description} \\ 
\specialrule{0.8pt}{0.0ex}{0.0ex}
$r$                 & The index of the restoration tasks \\
$b$                 & The index of adapter blocks \\
$l$                 & The index of adapter layers \\ 
\specialrule{0.8pt}{0.0ex}{0.0ex}
$E$                 & Easy subsets \\
$H$                 & Hard subsets \\ 
\specialrule{0.8pt}{0.0ex}{0.0ex}
Unet$_E$            & Unet trained with easy subsets of multiple restoration tasks \\
Unet$_{E+H}$        & Unet trained with easy and hard subsets of multiple restoration tasks \\ 
Unet-S$_E$          & Unet trained with an easy subset of single restoration task \\
Unet-S$_{E+H}$      & Unet trained with easy and hard subsets of single restoration task \\ 
\specialrule{0.8pt}{0.0ex}{0.0ex}
Restormer$_E$       & Restormer trained with easy subsets of multiple restoration tasks \\
Restormer$_{E+H}$   & Restormer trained with easy and hard subsets of multiple restoration tasks \\
Restormer-S$_E$     & Restormer trained with an easy subset of single restoration task \\
Restormer-S$_{E+H}$ & Restormer trained with easy and hard subsets of single restoration task \\ 
\specialrule{0.8pt}{0.0ex}{0.0ex}
PromptIR$_E$        & PromptIR trained with easy subsets of multiple restoration tasks \\
PromptIR$_{E+H}$    & PromptIR trained with easy and hard subsets of multiple restoration tasks \\
PromptIR-S$_E$      & PromptIR trained with an easy subset of single restoration task \\
PromptIR-S$_{E+H}$  & PromptIR trained with easy and hard subsets of single restoration task \\ 
\specialrule{0.8pt}{0.0ex}{0.0ex}
\multirow{2}{*}{AdaIR} & AdaIR fine-tuned with hard subset of target restoration task \\
& with frozen foundation model trained by easy subsets of multiple restorations tasks \\
\specialrule{0.8pt}{0.0ex}{0.0ex}
\multirow{2}{*}{AdaIR-S} & AdaIR fine-tuned with hard subset of target restoration task \\
& with frozen foundation model trained by an easy subset of single restorations task \\
\specialrule{0.8pt}{0.0ex}{0.0ex}
\end{tabular}
}
\caption{The list of notations.}
\label{table::notations}
\vspace{-15pt}
\end{table}
